# Supplementary material for: Verifying the Causes of Adversarial Examples
Source: arXiv:2010.09633 source file (2020-10-19)
Supplement: Supplementary file 1 [file appendix.tex]

\subsection{Preset Classification Benchmark}
We build a preset classification benchmark dataset based on MIT-Adobe FiveK dataset \cite{fivek}. In particular, we apply ten artistic presets using Adobe Camera Raw to the photos adjusted by expert C, generating a total of 11 styles (including the original ones). Example photos are shown in Fig. \ref{fig:preset-dataset}. 

\begin{figure}[h]
    \centering
    \includegraphics[width=\columnwidth]{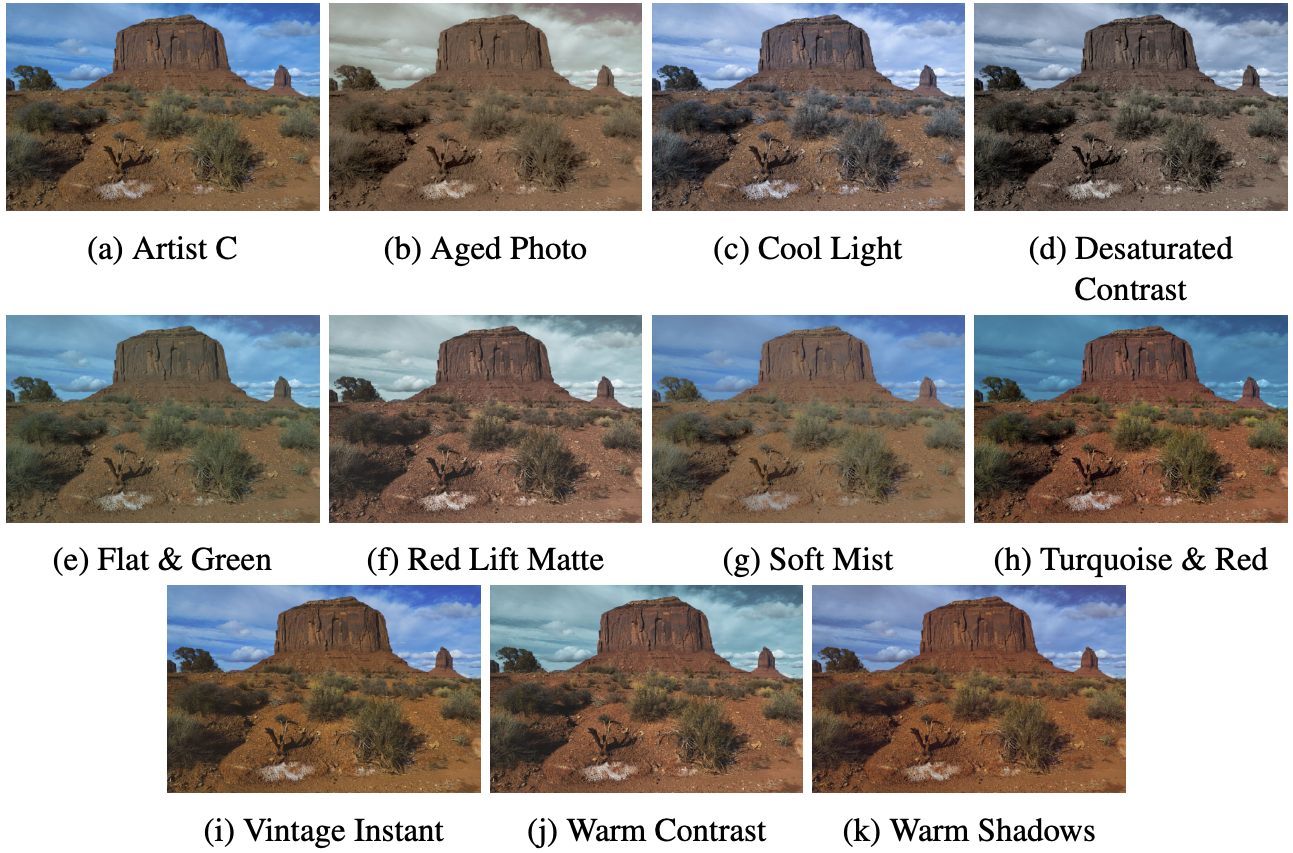}
    \caption{Sample photos from the preset dataset. }
    \label{fig:preset-dataset}
\end{figure}

\subsection{Excessive number of target categories for PNN and DE}
We also verify Hypothesis \ref{hyp:classes} using the proposed PNN and DE. Results from PNN and DE in Fig. \ref{fig:number-of-class_PNN-DE_result} show a similar trend as that in Fig. \ref{fig:number-of-class_result}. 
\begin{figure}[h]
    \centering
    \begin{subfigure}[b]{0.48\linewidth}
        \centering
        \includegraphics[width=\linewidth, height=3.6cm]{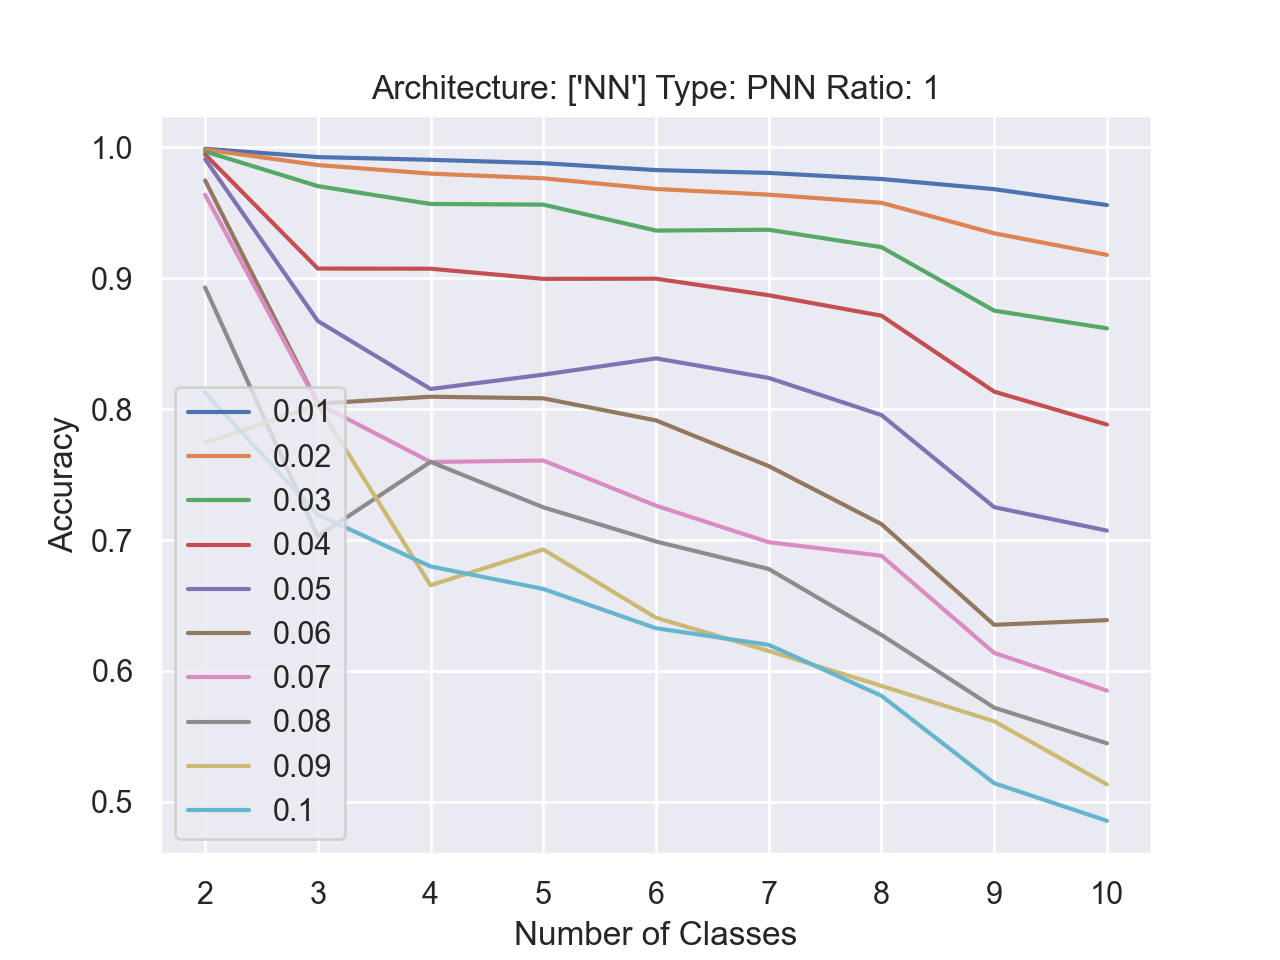}
        \caption{\centering PNN}
        \label{subfig:number-of-class_additive_PNN}
    \end{subfigure}
    ~
    \begin{subfigure}[b]{0.48\linewidth}
        \centering
        \includegraphics[width=\linewidth, height=3.6cm]{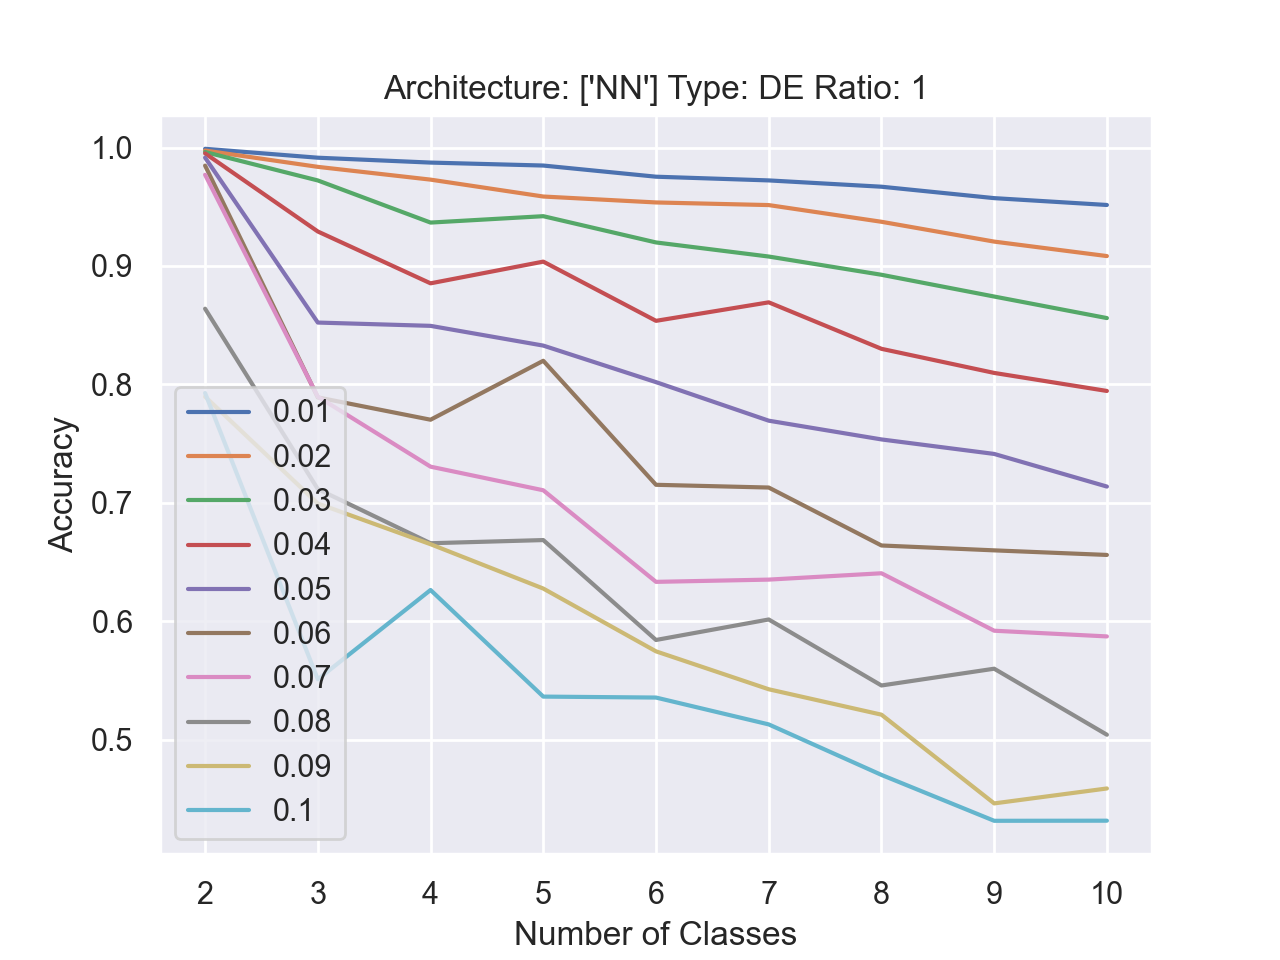}
        \caption{\centering DE}
        \label{subfig:number-of-class_constant_DE}
    \end{subfigure}
    
    \caption{Robustness of classifiers decreases as the number of target categories increases. $\epsilon$ (eps): the strength of attacks. }
    \label{fig:number-of-class_PNN-DE_result}
\end{figure}
